# Supplementary material for: Unconventional Growth Kinetics and Fractal Interfaces of Colloidal Phase Separation in Active Liquids
Source: arXiv:2508.11000 source file (2026-09-09)
Supplement: Supplementary file 1 [file SI.pdf]

# Supplementary Information for Unconventional Phase Separation and Fractal Interfaces of Colloids in Active Liquids

Pragya Kushwaha<sup>1</sup>, Pratikshya Jena<sup>2</sup>, Partha Sarathi Mondal<sup>2</sup>,  
Sanjay Puri<sup>4</sup>, Shradha Mishra<sup>2</sup>, and Vijayakumar Chikkadi<sup>1\*</sup>

<sup>1</sup> *Indian Institute of Science Education and Research( IISER) Pune, India 411008*

<sup>2</sup> *Indian Institute of Technology (BHU) Varanasi, India 221005 and*

<sup>4</sup> *Jawaharlal Nehru University (JNU),  
New Delhi, India 110067*

## CONTENTS

|                                                                                       |    |
|---------------------------------------------------------------------------------------|----|
| I. Experimental Methods                                                               | 2  |
| A. Experimental set-up                                                                | 2  |
| B. Constancy of effective diffusion coefficient in experiments                        | 2  |
| II. Robustness of coarsening exponent at varying densities of colloids and swimmers   | 3  |
| III. Theoretical modeling                                                             | 4  |
| A. Numerical details                                                                  | 4  |
| B. Phase separation kinetics                                                          | 5  |
| C. Finite size analysis                                                               | 8  |
| D. Dynamic scaling of the correlation function in simulations                         | 8  |
| E. Robustness of slow growth and rough interfaces                                     | 9  |
| IV. Movie files of the coarsening of colloidal domains in experiments and simulations | 10 |
| References                                                                            | 11 |

---

\* Corresponding authors : purijnu@gmail.com, smishra.phy@itbhu.ac.in, vijayck@iiserpune.ac.in

## I. EXPERIMENTAL METHODS

### A. Experimental set-up

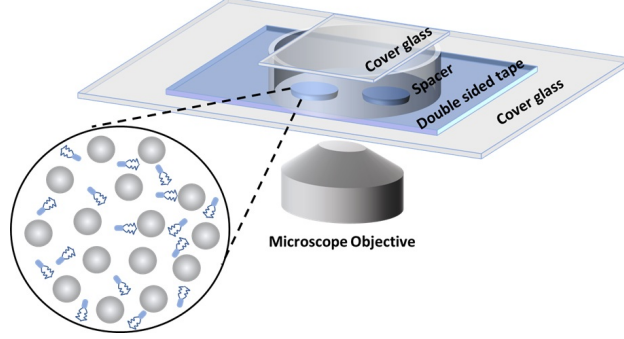

FIG. S1. Sketch of the sample chamber used in our experiments. The dimensions of the system are not to scale. The double-sided tape has a thickness of  $100\mu m$  and it has two circular cavities. One of them is filled with the suspension of colloidal particles and E. coli, and the other cavity contains DI water. The cover glass on top of the spacer minimizes the evaporation losses.

The observation chamber was constructed using double-sided tape with a circular cavity of  $1cm$  diameter and  $100\mu m$  depth, which was glued to a PEG-coated coverlip. A sketch of the sample chamber is shown in Fig. S1. The dimensions of the system are not to scale. We use double-sided tape with two cavities. One of the cavities is filled with the suspension of colloidal particles and E. coli, while the other contains deionized water. The cover glass on top of the spacer minimizes evaporation losses and has small openings in two corners to prevent oxygen depletion, as shown in the schematic diagram.

### B. Constancy of effective diffusion coefficient in experiments

As our experiments are conducted over a maximum duration of 210 – 250 minutes, we calculated the effective diffusion constant  $D_{\text{eff}}$  to ensure that the bacterial activity remains constant over this duration. The effective diffusion constant  $D_{\text{eff}}$  in our study is calculated using the expression [1]

$$D_{\text{eff}} = \frac{1}{4} \frac{\delta \langle \Delta r^2(t) \rangle}{\delta t}.$$

The  $D_{\text{eff}}$  is determined at different times starting from the beginning of the experiment and the results are shown in Fig. S2 at dilute densities of colloidal particles corresponding to an

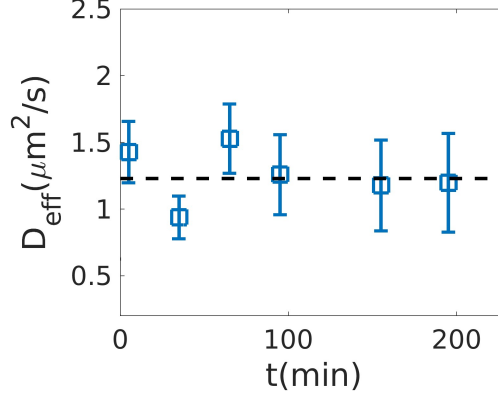

FIG. S2. The effective diffusion constant  $D_{\text{eff}}$  of colloidal particles in active liquids at a bacteria concentration  $c_b = 5b_0$ . The area fraction of colloids is  $\rho_0 = 0.005$ . The dashed line indicates the mean value. The error bars are obtained from the standard deviations of  $D_{\text{eff}}$ .

area fraction  $\rho_0 \sim 0.005$  and a swimmer density of  $c_b = 5b_0$ . The estimate of  $D_{\text{eff}}$  fluctuates around a mean value, suggesting constancy of the swimmer activity over the duration of the experiment.

## II. ROBUSTNESS OF COARSENING EXPONENT AT VARYING DENSITIES OF COLLOIDS AND SWIMMERS

To confirm the robustness of the coarsening exponent associated with the growth of colloidal clusters, we have determined the length scale  $L(t)$  for various area-fractions of colloids,  $\rho_0 = 0.1, 0.2$ , and  $0.3$ , at a fixed bacterial density of  $c_b = 5b_0$ , as shown in Figs. S3(a)–(c). We have also determined  $L(t)$  for different bacterial densities,  $c_b = 1b_0, 5b_0$ , and  $10b_0$ , at a fixed area fraction  $\rho_0 \sim 0.2$  of colloids, as shown in Figs. S3(d)–(e). The red line corresponds to a slope of  $1/4$ , while the black line has a slope of  $1/3$ . The length scale  $L(t)$  was extracted from the spatial correlation function of the order parameter  $\phi$ , as described in the main text. These results clearly demonstrate that a growth exponent of  $1/4$  is robust across a range of colloidal area fractions and bacterial concentrations.

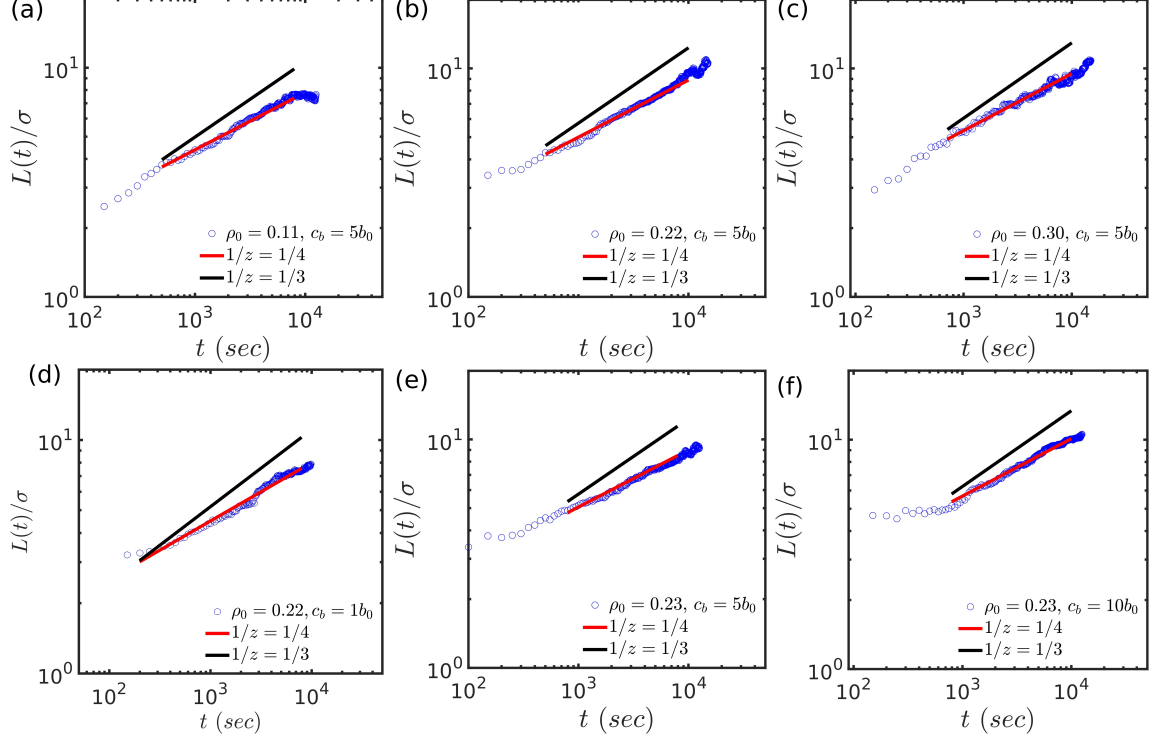

FIG. S3. Upper panels (a)–(c): Length scale  $L(t)$  at various area fractions of colloids corresponding to  $\rho_0 = 0.1, 0.2$ , and  $0.3$ , respectively, and a fixed bacterial density of  $c_b = 5b_0$ . Lower panels (d)–(e): Length scale  $L(t)$  at various bacterial densities  $c_b = 1b_0, 5b_0$ , and  $10b_0$  for a fixed area fraction  $\rho_0 \sim 0.2$ . The red and black lines have slopes of  $1/4$  and  $1/3$ , respectively.

### III. THEORETICAL MODELING

#### A. Numerical details

We numerically integrate equation of Model B (MB) with colored noise

$$\frac{\partial \phi(\mathbf{r}, t)}{\partial t} = \nabla^2 (-\phi + \phi^3 - \nabla^2 \phi) + \nabla \cdot \xi, \quad (1)$$

where the simplest spatio-temporally correlated colored noise  $\xi(\mathbf{r}, t)$  can be obtained by solving the linear second order reaction-diffusion equation [2, 3]:

$$\frac{\partial}{\partial t} \xi(\mathbf{r}, t) = -\frac{1}{\tau} (1 - \lambda^2 \nabla^2) \xi(\mathbf{r}, t) + \frac{1}{\tau} \eta(\mathbf{r}, t). \quad (2)$$

The units of space and time in Eq. (2) are the dimensionless units introduced in the main manuscript. The spatial correlation length  $\lambda$  and timescale  $\tau$  of the noise arises from the Laplacian term, which couples the values of the field  $\xi(\mathbf{r}, t)$  at different points. In Eq. (2),

$\eta(\mathbf{r}, t)$  is a Gaussian white noise with zero average and correlation

$$\langle \eta(\mathbf{r}, t) \eta(\mathbf{r}', t') \rangle = 2\epsilon \delta(\mathbf{r} - \mathbf{r}') \delta(t - t'), \quad (3)$$

where the strength  $\epsilon = 5$  in our simulations. We also checked the results for larger  $\epsilon = 25, 50$  and this only affects prefactors.

Eqs. (1) and (2) are numerically integrated using the Euler scheme with  $\Delta x = 1.0$  and  $\Delta t = 0.005$ . The system is a two dimensional box of size  $K \times K$  with periodic boundary condition in both directions. To stabilize the contribution of the Laplacian, we require [2]

$$\frac{4\lambda^2}{\tau} \times \frac{\Delta t}{(\Delta x)^2} < 1. \quad (4)$$

The size of the system  $K$  is varied from 256 – 2048, and the total simulation time  $t_s = 50000$  with the actual time being  $t_s \times \Delta t = 250$ . One simulation time consists of a single update of the equations for  $\phi$  Eq. (7) (in the main manuscript) and  $\xi$  in Eq. (2) for all lattice points. The magnitudes of  $\lambda$  and  $\tau$  in our simulations are chosen in light of experimental inputs. The persistence time of colloidal beads shows minimal change, whereas their persistence length experiences small but noticeable variations with bacterial density. Hence we perform our simulations with  $\tau = 1$ . The parameter  $\lambda$  is varied between 0-7 to mimic the effect of variation in bacterial density.

We start from a disordered homogeneous state at  $t = 0$  with small-amplitude fluctuations:  $\phi(\mathbf{r}, 0) = \phi_0 + \delta\phi(\mathbf{r}, 0)$ . The corresponding mean density is  $\rho_0 = (1 + \phi_0)/2$ . The coupled system of partial differential equations for  $\phi$  and  $\xi$  are evolved to obtain configurations of the order parameter. The ordering kinetics is characterized by evolution of morphologies, correlation functions, and structure factors as defined in Eqs. (1) and (2) in the main manuscript. All statistical quantities reported here are obtained as an average over 50 – 100 independent runs.

## B. Phase separation kinetics

The mean density of the particles is kept to low values  $\rho_0 = 0.05, 0.1, 0.15$  with the corresponding values of  $\phi_0 = -0.9, -0.8, -0.7$ , respectively. In Fig. S4, we show the evolution

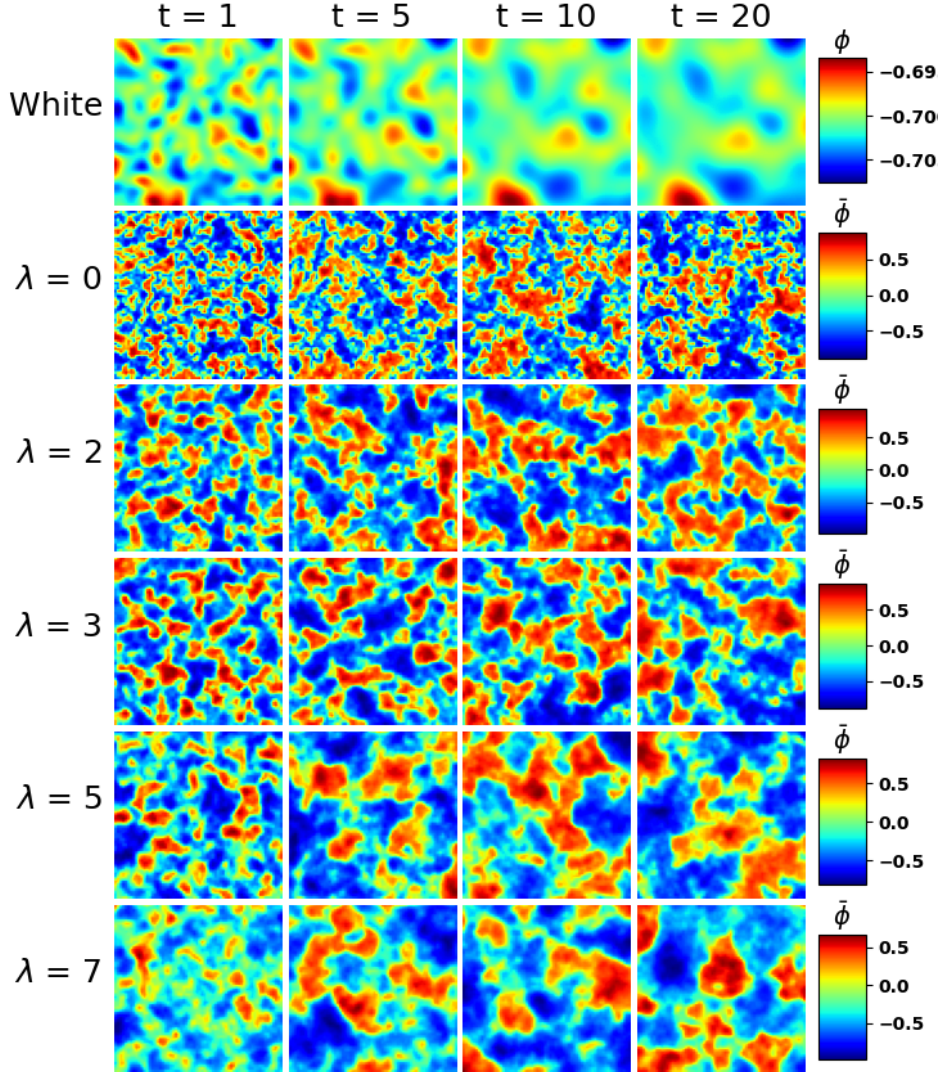

FIG. S4. The panels display the phase diagram in plane of  $\lambda$  and time. From left to right, the panels depict the evolution of local order parameter  $\phi(\mathbf{r})$  (for White noise) and normalized local order parameter  $\bar{\phi}(\mathbf{r})$ . The correlation length is varied over the range  $\lambda = 0 - 7$ . The mean density of the system is  $\rho_0 = 0.15$ . See section III B for the definition of  $\bar{\phi}$ .

of the normalized local order parameter  $\bar{\phi}(\mathbf{r}, t)$  in the system for different cases.  $\bar{\phi}(\mathbf{r}, t)$  is obtained by dividing local order parameter,  $\phi(\mathbf{r}, t) = 2\rho_l(r, t) - 1$ , with the maximum of  $|\phi|$  in the system. From left to right in the figure, the snapshots are depicted at different times, as shown for the mean density  $\rho_0 = 0.15$ . From top to bottom, we show snapshots for the system with white noise (Model B or MB) and colored noise with different  $\lambda$ . For MB (top panel), the snapshots are of the order parameter field  $\phi$  and represent the weak density



inhomogeneity in the system. For MB at the high off-criticality considered here ( $\phi_0 = 0.7$ ), growth occurs by nucleation of droplets. There is no significant nucleation on the short time-scales of our simulation in Fig. S4. MB with colored noise shows small domains for  $\lambda \leq 3$  and domain growth is more prominent for  $\lambda \geq 5$ .

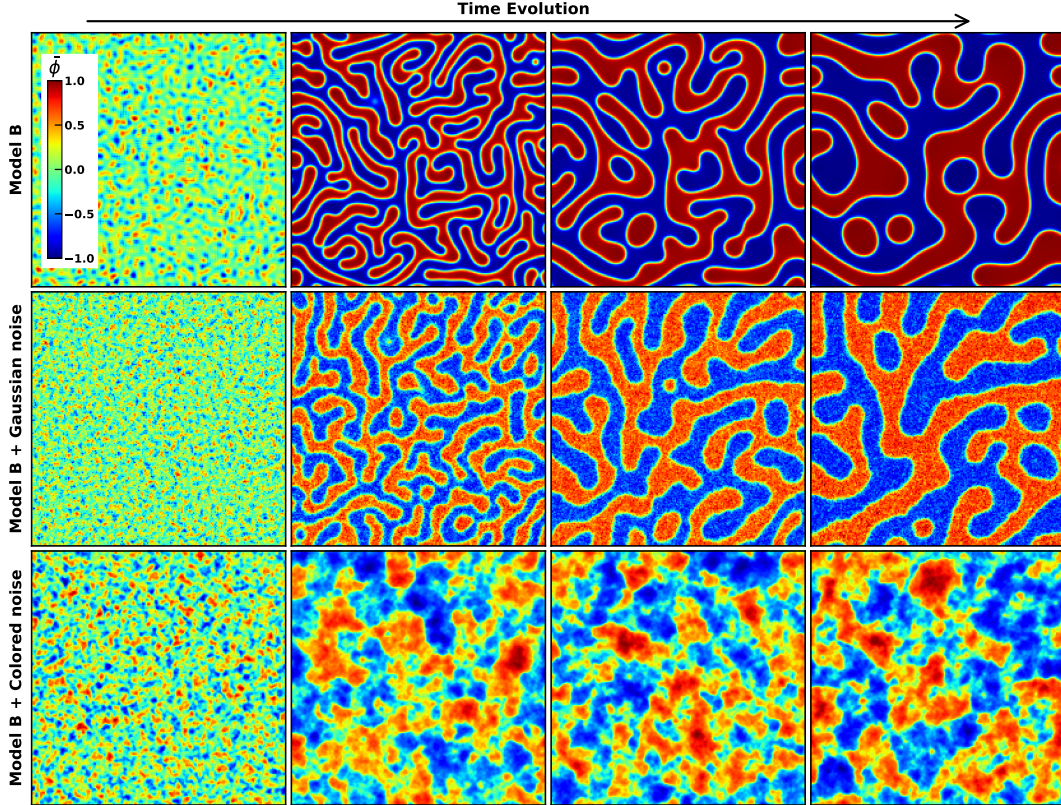

FIG. S5. The panels display the time evolution of the order parameter field for the MB with critical composition  $\phi_0 = 0$ ; (a) without noise, (b) with Gaussian white noise and (c) with colored noise ( $\tau = 1, \lambda = 7$ ). The different columns are for different times 100, 500, 1000 and 2000. The color bar have the same meaning as in Fig. S4. See section III B for the definition of  $\bar{\phi}$ .

For comparison, in Fig. S5, we show instantaneous snapshots of phase-separating domains for MB with critical composition ( $\psi_0 = 0$ ) in three different cases: (i) MB without thermal noise, (ii) MB with Gaussian white noise, and (iii) MB with colored noise ( $\tau = 1, \lambda = 7$ ). In Fig. S5, from left to right, we show snapshots for different times: 100, 500, 1000, 2000. The domain morphology is very different for MB with colored noise in comparison to cases (i)

and (ii). In particular, the domain walls are rough and fuzzy, suggesting a fractal nature. This is reflected in the non-Porod behavior of the correlation functions and structure factors, shown in the main manuscript. We have confirmed that the fractal dimension of the domain walls ( $d_f \simeq 1.34$ ) is robust for a wide range of parameter values.

### C. Finite size analysis

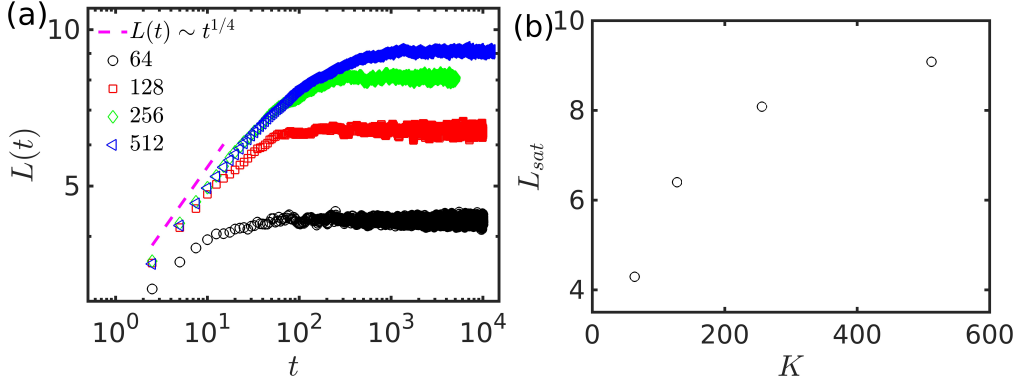

FIG. S6. (color online) The plot showcase the finite size analysis of  $L(t)$  vs.  $t$  at late times. (a) The plot of  $L(t)$  vs.  $t$  for four different  $K = 64, 128, 256$  and  $512$ . The dashed line is  $L(t) \sim t^{1/4}$ . (b) Plot of  $L_{sat}$  vs.  $K$ .

Our simulations reveal that the growth of domains is arrested on longer timescale, leading to saturation of the domain size. However, such a saturation can also arise due to finite size effects. To illuminate these aspects, we perform the finite size analysis of  $L(t)$  for different system sizes  $K = 64, 128, 256$  and  $512$ . In Fig. S6(a) we show the  $L(t)$  vs.  $t$  for four different system sizes. At early times the  $L(t) \sim t^{1/4}$  and shows a clear saturation at late times. Further we claim that such saturation is not due to the finite size effect. In Fig. S6(b) we show the  $L_{sat}$  vs.  $K$ , where  $L_{sat}$  is defined as the late time saturated  $L(t)$ .  $L_{sat}$  flattens with  $K$  at large  $K$ , which represents microphase separation in the system.

### D. Dynamic scaling of the correlation function in simulations

The Fig. S7 presents the two different scalings of the correlation function  $C(r, t)$ . The collapse of the data is better when  $C(r, t)$  is scaled using  $t^{1/4}$ , instead of  $t^{1/3}$ .



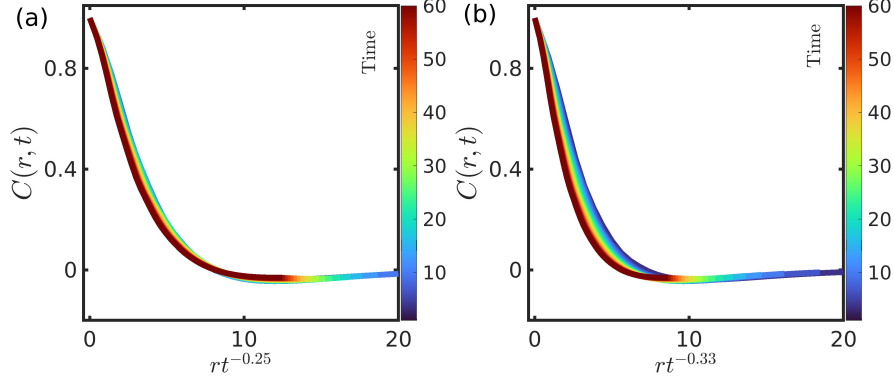

FIG. S7. Dynamic scaling and slow growth of the correlation function  $C(r, t)$ . The function  $C(r, t)$  in panels (a) and (b) are scaled by  $t^{1/4}$  and  $t^{1/3}$ , respectively. The color bar represents the time progression. The data are obtained from a simulation box of size  $K = 1024$ .

### E. Robustness of slow growth and rough interfaces

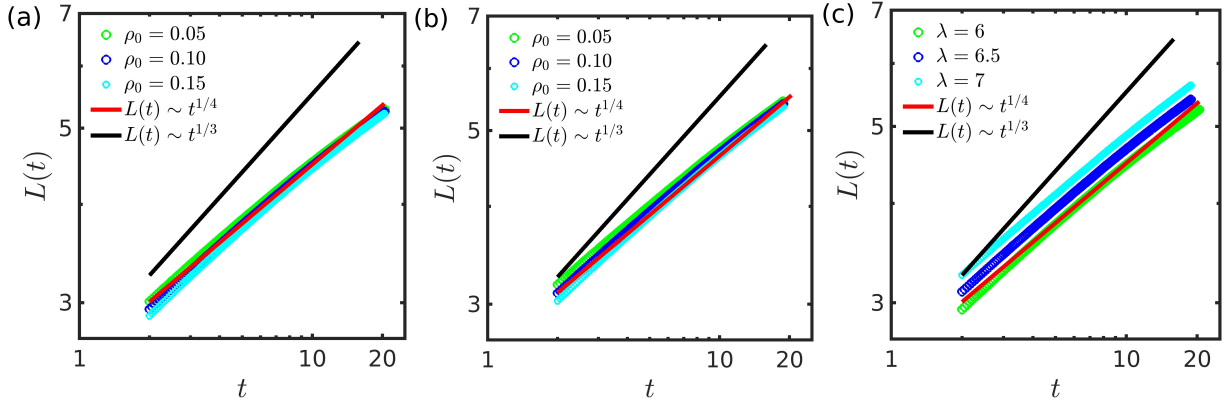

FIG. S8. Growth of the coarsening length scale  $L(t)$  at  $\rho_0 = 0.05, 0.1, 0.15$  and the set  $\lambda = 6.0$  and  $6.5$  are shown in (a) and (b), respectively. The dotted magenta line and cyan line show the slope  $0.33$  and  $0.25$  respectively. The plot (c) shows the same plot for fixed  $\rho_0 = 0.1$  and  $\lambda = 6.0, 6.5$  and  $7.0$ . The lines have the same slopes as in (a) and (b).

In this section, we present the robustness of the growth law found in our simulations. The Figs. S8(a) display the growth of  $L(t)$  at  $\rho_0 = 0.05, 0.1$ , and  $0.15$  and  $\lambda = 6.0$ , while the panel in (b) the results for  $\lambda = 6.5$  is shown. The Fig. S8(c) presents  $L(t)$  for varying  $\lambda = 6, 6.5$  and  $7$  at  $\rho_0 = 0.1$ . We also demonstrate that the interfaces remain rough over a range of parameters investigated in our simulations. The Fig. S9 shows the scaled of structure factor  $L^{-2}(t)S(k)$  for  $\lambda = 6.5$  and  $7.0$ . The strong non-Porod scaling of the struc-

ture factor shows that rough interfaces are characteristic features of phase separation in the presence of colored noise. These results are supported by the visual impression of the domains presented in Fig. S4.

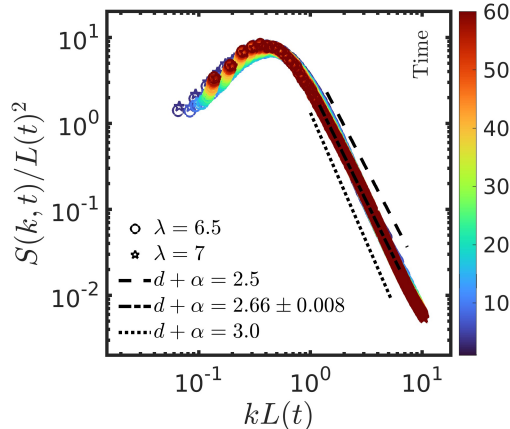

FIG. S9. The scaled structure factor  $L^{-2}(t)S(k)$  is plotted against  $kL(t)$  for Model B with colored noise for  $\lambda = 6.5$  and  $7.0$ .

#### IV. MOVIE FILES OF THE COARSENING OF COLLOIDAL DOMAINS IN EXPERIMENTS AND SIMULATIONS

The supplementary information contain videos of the coarse-grained hardened order parameter field  $\phi(\mathbf{r}, t)$  obtained from experiments and simulations. The order parameter  $\phi$ , is color-coded, with its magnitude varying from  $+1$  to  $-1$ . The information about the video files is given below :

SM1: Formation of colloidal domains in the experiments over a duration of 210 minutes. The area fraction of colloids is  $\rho_0 = 0.28$  and the concentration of the swimmers is  $c_b = 5b_0$ . The playback speed has been accelerated to present the slow process of colloidal ordering.

SM2: Phase separation kinetics of colloidal domains in experiments. The video captures the evolution of  $\phi$  over a timescale of 210 minutes, beginning from the homogeneous phase at the start of the experiment. The bacterial density is  $c_b = 5b_0$ , and the colloidal area fraction

is  $\rho_0 = 0.28$ .

SM3: Phase separation kinetics of domains in simulations with spatio-temporally correlated noise. The video shows the evolution of the system from the initial homogeneous phase at  $t = 0$  to the phase-separated state at  $t = 30$ . The order parameter  $\phi$  is color-coded. Parameters used in the simulation are: average density  $\rho_0 = 0.15$ , system size  $K = 512$ , noise correlation length  $\lambda = 7$ , and correlation time  $\tau = 1$ .

SM4: Late time video of domains in simulations with spatio-temporal noise ( $t = 30$  to  $60$ ). Other parameters are the same as in SM3.

SM5: Phase separation kinetics of domains in Model B with Gaussian white noise. The video shows the system evolution from  $t = 40$  to  $t = 60$  for a critical composition  $\phi_0 = 0$  and system size  $K = 512$ .

For better resolution and clarity only a part of the full system is shown in SM3 - SM5.

- 
- [1] X.-L. Wu and A. Libchaber, Particle diffusion in a quasi-two-dimensional bacterial bath, Physical review letters **84**, 3017 (2000).
  - [2] J. García-Ojalvo, J. M. Sancho, and L. Ramirez-Piscina, Generation of spatiotemporal colored noise, Physical Review A **46**, 4670 (1992).
  - [3] F. Sagués, J. M. Sancho, and J. García-Ojalvo, Spatiotemporal order out of noise, Reviews of Modern Physics **79**, 829 (2007).
